# Supplementary material for: Pressure-driven collapse of the relativistic electronic ground state in a honeycomb iridate
Source: arXiv:1803.04056 source file (2018-03-11)
Supplement: Supplementary file 1 [file HP_213_supplemental_arXiv.pdf]

# Supplemental Material: Pressure-driven collapse of the relativistic electronic ground state in a honeycomb iridate

J. P. Clancy,[1] H. Gretarsson,[1] J. A. Sears,[1] Yogesh Singh,[2] S. Desgreniers,[3] Kavita Mehlawat,[2] Samar Layek,[4] Gregory Kh. Rozenberg,[4] Yang Ding,[5] M. H. Upton,[6] D. Casa,[6] N. Chen,[7] Junhyuck Im,[8] Yongjae Lee,[8,9] R. Yadav,[10] L. Hozoi,[10] D. Efremov,[10] J. van den Brink,[10] and Young-June Kim[1]

[1]*Department of Physics, University of Toronto, Toronto, Ontario M5S 1A7, Canada*
[2]*Indian Institute of Science Education and Research Mohali, Sector 81, SAS Nagar, Manauli PO 140306, India*
[3]*Laboratoire de physique des solides denses, Department of Physics, University of Ottawa, Ottawa, Ontario, K1N 6N5, Canada*
[4]*School of Physics and Astronomy, Tel Aviv University, 69978 Tel Aviv, Israel*
[5]*Center for High-Pressure Science & Technology Advanced Research (HPSTAR), Beijing, 100094, China*
[6]*X-ray Science Division, Advanced Photon Source, Argonne Nation Laboratory, Argonne, Illinois 60439, USA*
[7]*Canadian Light Source, Saskatoon, Saskatchewan, S7N 0X4, Canada*
[8]*Department of Earth System Sciences, Yonsei University, Seoul 120-749, Korea*
[9]*Center for High Pressure Science & Technology Advanced Research (HPSTAR), Shanghai 201203, China*
[10]*Institute for Theoretical Solid State Physics, IFW Dresden, Helmhotzstr. 20, 01069 Dresden, Germany*

## EXPERIMENTAL DETAILS

X-ray absorption spectroscopy measurements were performed using the Hard X-Ray MicroAnalysis (HXMA) beamline 06ID-1 at the Canadian Light Source. Data was collected in fluorescence yield detection mode, using a 32 element Ge detector. The incident energy was selected using a Si (111) monochromator, and the higher harmonic contributions were suppressed by a combination of Rh-coated mirrors and a 50% detuning of the wiggler.

X-ray powder diffraction measurements were performed using HXMA at the CLS. Data was collected with angle dispersive techniques [1], using high energy x-rays ($E_i$ = 24.35 keV, $\lambda$ = 0.509176 Å) and a MAR345 image plate detector. Full Rietveld refinements were performed using the GSAS software package [2].

Resonant inelastic x-ray scattering measurements were performed using the MERIX spectrometer on beamline 30-ID-B at the Advanced Photon Source. A diamond (111) primary monochromator, silicon (220) secondary monochromator, and spherical (2 m radius) diced silicon (844) analyzer were used to produce a high flux, medium resolution instrument configuration. The overall energy resolution [full width at half maximum (FWHM)] in this configuration was 110 meV. In order to minimize the elastic background intensity, measurements were carried out in horizontal scattering geometry with a scattering angle close to $2\theta = 90°$.

All measurements were performed at room temperature. Loose powder samples were loaded into a diamond anvil cell, using either panoramic (XAS, RIXS) or transmission (XRD) cell geometries. The pressure was tuned with a precision of ±0.2 GPa using the R1 fluorescent line from a ruby chip placed inside the sample space. To ensure reproducibility, high pressure measurements were repeated using a series of different pressure transmitting media. XAS measurements were carried out using low viscosity silicone fluid, XRD measurements were carried out using high viscosity silicone fluid, nitrogen gas, and water, and RIXS measurements were carried out using neon gas. Over these pressure ranges, all four pressure transmitting media are expected to deliver reasonable, quasi-hydrostatic performance. The reversibility of the pressure-induced changes was verified by performing measurements at partial and full pressure release after the highest pressure data points had been collected. Due to the presence of hysteresis effects associated with the first order structural transition at 3 GPa, all measurements presented here have been obtained under increasing pressure conditions (unless explicitly stated otherwise).

## FIRST PRINCIPLES CALCULATIONS

Density functional theory (DFT) calculations were carried out within the local (spin) density approximation [L(S)DA] using the Full Potential Local Orbital band structure Package (FPLO) [3]. A k-mesh of 6×6×6 k-points in the whole Brillouin zone was employed. In order to account for correlation effects in the Ir 5d-shell we adopted the L(S)DA+U scheme. Due to the rather sizable spin-orbit interaction of the Ir atoms the full relativistic four-component Dirac scheme was used.

Similar to other iridates, the LDA results suggest a metallic state. To obtain an insulating ground state one needs to take into account strong correlations in mean field approximation (LDA+U). We introduce a Hubbard $U = 2.0$ eV and Hund's coupling of $J = 0.5$ eV for the Ir 5d-shell.

In order to extract theoretical values for the Ir $L_3/L_2$

branching ratio, the quantity which is experimentally probed by XAS, *ab initio* calculations were performed using many-body quantum chemistry methods. These calculations were performed on a finite cluster of atoms consisting of one $IrO_6$ reference octahedron, four nearest-neighbor (NN) $IrO_6$ octahedra, and fifteen adjacent Li ions. The latter accounts for the finite charge distribution in the immediate neighborhood of the central $IrO_6$ unit. The remaining part of the lattice was modeled by point charges fit to reproduce the ionic Madelung potential in the cluster region. Energy-consistent relativistic pseudopotentials and basis functions of quadruple-zeta quality [4] were used to describe the valence shell of the central Ir ion, while all-electron basis sets of triple-zeta quality [5] were applied for the ligands corresponding to the reference octahedron. The NN Ir ions were represented by closed-shell $Pt^{4+}$ $t_{2g}^6$ species, using relativistic pseudopotentials and triple-zeta basis functions for the valence shell [4]. For the oxygen sites corresponding to the NN octahedra, all-electron minimal atomic-natural-orbital basis sets were employed [6]. Total-ion effective potentials along with a single $s$ valence function were used for the adjacent Li species [7].

All computations were carried out with the MOLPRO quantum chemistry package [8]. Multiconfigurational wave functions were first obtained using the complete-active-space self-consistent-field (CASSCF) approach. The CASSCF optimization was carried out for an average of the $^2T_{2g}$ $(t_{2g}^5)$, $^4T_{1g}$ $(t_{2g}^4e_g^1)$, $^4T_{2g}$ $(t_{2g}^4e_g^1)$, and $^6A_{1g}$ $(t_{2g}^3e_g^2)$ states. In the final multireference configuration-interaction (MRCI) calculations [9, 10], single and double excitations were allowed from the O $2p$ and Ir $5d$ orbitals of the reference octahedron. All the aforementioned states entered the spin-orbit treatment, carried out as described in Ref. [11]. The branching ratios were derived at the MRCI level, following the procedure described in Ref. [12].

Representative crystal structures determined from XRD measurements at ambient pressure, 0.1 GPa, 0.6 GPa, and 2.8 GPa were used as input for the quantum chemistry calculations. The resulting MRCI branching ratios are plotted in the inset of Figure 1 in the main text. It is clear that the computed values capture the same qualitative trend as the experimental data but systematically underestimate the observed branching ratios. It has been shown that better agreement with the experimental data can be obtained by including more excited states in the spin-orbit treatment [12], however, this aspect of the calculation falls beyond the scope of the present study.

## HIGH PRESSURE RESISTIVITY MEASUREMENTS

High pressure electrical resistance measurements on $\alpha$-$Li_2IrO_3$ are shown in Supplemental Figure 1. The main panel illustrates the temperature dependence of the resistivity at three representative pressures: ambient (within the undistorted monoclinic/high branching ratio phase), P = 1.5 GPa (within the slightly distorted monoclinic/low branching ratio phase) and P = 7 GPa (within the highly distorted triclinic/low branching ratio phase). At fixed pressure the resistance data fairly accurately obey the relation $\ln(R) \sim (T_0/T)^{1/4}$ (see the upper inset) consistent with the Mott variable-range hopping law [13, 14], where $T_0$ is the Mott temperature. The pressure dependence of the room temperature resistance (T = 298 K) is shown in the lower inset. These measurements indicate that the electrical resistivity and the Mott temperature of $\alpha$-$Li_2IrO_3$ decrease slightly as a function of pressure, but that the system remains insulating in both the slightly distorted monoclinic phase and the highly distorted triclinic phase. As a result, it follows that the rapid pressure-induced drop in branching ratio coincides with the collapse of the $J_{eff}$ = 1/2 relativistic state, but not the destruction of the insulating ground state. These results are fully consistent with the DFT calculations presented in Figure 4 of the main text, and support the proposed transition between localized $J_{eff}$ = 1/2 and itinerant QMO regimes at P ∼ 0.1 GPa.

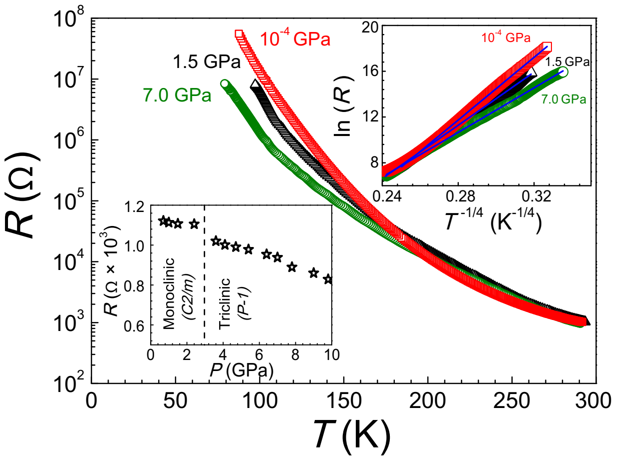


FIG. 1: (Color online) Pressure dependence of the electrical resistance of $\alpha$-$Li_2IrO_3$. Main panel: Resistance as a function of temperature for various pressures. The data for different samples, pressurized and at ambient pressure, are normalized to room temperature. Top inset: Temperature dependence of the resistance replotted as ln(R) vs. $T^{-1/4}$. Bottom inset: Room temperature resistivity as a function of pressure. Note the resistance drop at the transition from the monoclinic $C2/m$ phase to the triclinic $P$-$1$ phase.

## HIGH PRESSURE STRUCTURAL REFINEMENTS

The pressure dependence of the crystal structure of $\alpha$-$Li_2IrO_3$ was determined from Rietveld refinements performed using the GSAS software package [2]. The lattice parameters ($a$, $b$, $c$, $\alpha$, $\beta$, $\gamma$), positional parameters, thermal parameters ($U_{iso}$), background, and lineshape parameters were all individually, and then simultaneously, refined. In order to account for the effects of stacking disorder within the layered crystal structure, we also refined the occupancy of the Li 2a (0, 0, 0)and Ir 4g (0, y, 0) sites (i.e. using Li/Ir site disorder to mimic stacking faults, as done in previous work by O'Malley et al [15]). The occupancy was freely refined, then refined under the constraint that Occ[Li(2a)] + Occ[Ir(2a)] = 1 and Occ[Ir(4g)] + Occ[Li(4g)] = 1. No significant difference in the quality of refinement was observed for these two methods. Data was collected on four different powder samples of $\alpha$-$Li_2IrO_3$, and the level of stacking sequence disorder was found to range from 5% to 19%.

For data sets collected below 3 GPa, refinements were performed using a single phase and a monoclinic *C2/m* structural model. For data sets above 5 GPa, refinements were performed using a single phase and a triclinic *P-1* structural model. In the phase coexistence region between 3 to 5 GPa, a two phase refinement was performed using both structural models.

A series of representative refinements are provided in Supplemental Figure 2. These refinements were carried out on diffraction patterns collected at pressures of P = 2.8 GPa ( within the lightly distorted monoclinic phase) and P = 5.2 GPa (within the heavily distorted triclinic phase) using low viscosity silicone fluid [1ct polydimethylsiloxane] as a pressure transmitting medium. Structural parameters from representative refinements performed at ambient pressure, P = 0.1 GPa, 2.8 GPa, and 5.2 GPa are provided in Tables 1, 2, and 3. Note that the ambient pressure refinement results were previously reported by our group in an earlier study [16].

The pressure dependence of the lattice parameters for $\alpha$-$Li_2IrO_3$ is illustrated in Supplemental Figure 3. These parameters reveal: (i) a sharp, discontinuous change in unit cell lengths and unit cell angles at 3 GPa, (ii) a clear deviation from monoclinic symmetry above 5 GPa, and (iii) an extended region of phase coexistence from 3 to 5 GPa where both phases are present.

It should be noted that accurate refinement of the atomic positions for the lighter Li and O atoms becomes increasingly difficult at higher pressures. This is due to a combination of two main effects: (i) the large difference in electronic charge density between Ir (Z = 77) and Li (Z = 3) and O (Z = 8), which limits x-ray sensitivity to the lighter atoms, and (ii) significant lineshape broadening which arises due to pressure-induced strain effects. Although accurate positional refinements are still pos-

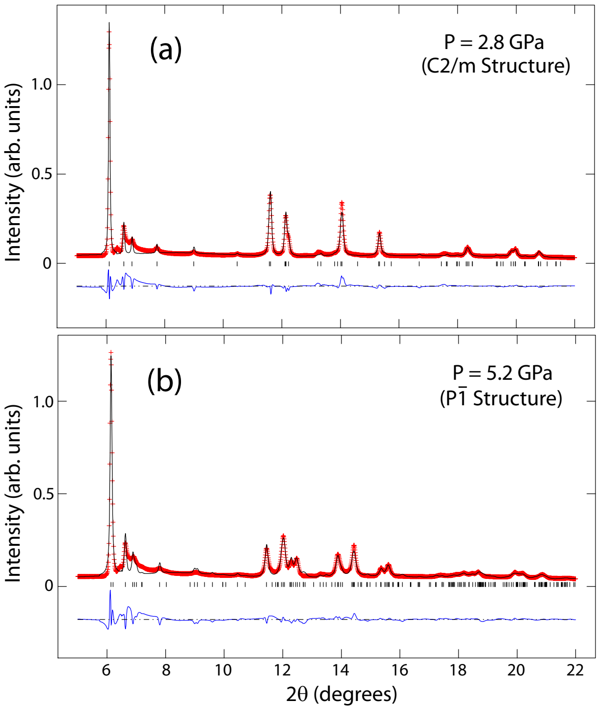


FIG. 2: (Color online) Representative Rietveld refinements for $\alpha$-$Li_2IrO_3$ at P = 2.8 GPa (*C2/m* phase) and 5.2 GPa (*P-1* phase). Data points are represented by the red crosses, the Rietveld fit is represented by the solid black line, and the difference is represented by the solid blue line.

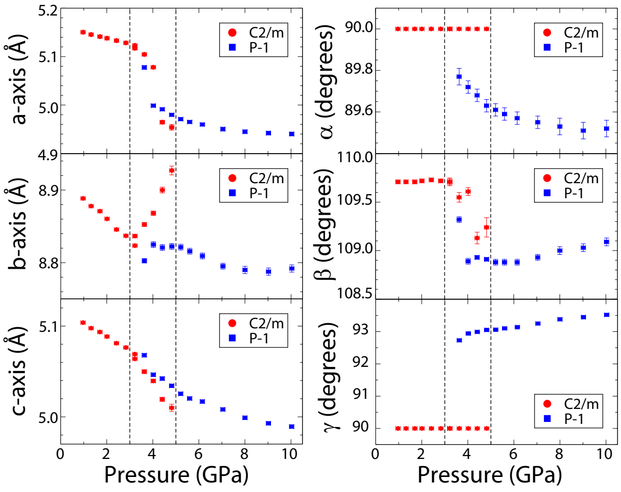


FIG. 3: (Color online) Pressure dependence of the lattice parameters for $\alpha$-$Li_2IrO_3$. Parameters have been extracted from Rietveld refinements performed on high pressure x-ray diffraction data, as shown in Figure 2 of the main text. Note the presence of the discontinuous transition at P $\sim$ 3 GPa, and the extended phase coexistence region which extends up to P $\sim$ 5 GPa.

TABLE I: Lattice parameters for $\alpha$-$Li_2IrO_3$ at several representative pressures.

| | Ambient [16] | P = 0.1 GPa | P = 2.8 GPa | P = 5.2 GPa |
|---|---|---|---|---|
| Space Group | *C2/m* | *C2/m* | *C2/m* | *P-1* |
| a (Å) | 5.172(1) | 5.167(1) | 5.128(1) | 4.971(1) |
| b (Å) | 8.926(2) | 8.899(1) | 8.837(1) | 8.821(2) |
| c (Å) | 5.122(2) | 5.107(1) | 5.076(1) | 5.025(1) |
| $\alpha$ (°) | 90 | 90 | 90 | 89.61(3) |
| $\beta$ (°) | 109.91(4) | 109.74(1) | 109.72(2) | 108.88(3) |
| $\gamma$ (°) | 90 | 90 | 90 | 93.06(2) |

TABLE II: Structural parameters for $\alpha$-$Li_2IrO_3$ in the low pressure monoclinic phase (P = ambient, 0.1 GPa, and 2.8 GPa).

| | Ambient [16] | P = 0.1 GPa | P = 2.8 GPa |
|---|---|---|---|
| Ir1 (4g) | (0, 0.333, 0) | (0, 0.326, 0) | (0, 0.322, 0) |
| Li1 (2a) | (0, 0, 0) | (0, 0, 0) | (0, 0, 0) |
| Li2 (2d) | (0, 0.5, 0.5) | (0, 0.5, 0.5) | (0, 0.5, 0.5) |
| Li3 (4h) | (0, 0.81, 0.5) | (0, 0.76, 0.5) | (0, 0.76, 0.5) |
| O1 (8j) | (0.248, 0.327, 0.769) | (0.239, 0.300, 0.724) | (0.245, 0.293, 0.695) |
| O2 (4i) | (0.293, 0, 0.740) | (0.281, 0, 0.812) | (0.327, 0, 0.809) |

TABLE III: Structural parameters for $\alpha$-$Li_2IrO_3$ in the high pressure triclinic phase (P = 5.2 GPa).

| | | | |
|---|---|---|---|
| Ir1 (2i) | (-0.041, 0.314, 0.041) | Ir2 (2i) | (0.459, 0.814, -0.041) |
| Li1 (1a) | (0, 0, 0) | Li2 (1e) | (0.5, 0.5, 0) |
| Li3 (1f) | (0.5, 0, 0.5) | Li4 (1g) | (0, 0.5, 0.5) |
| Li5 (2i) | ((0, 0.76, 0.5) | Li6 (2i) | (0.5, 0.26, 0.5) |
| O1 (2i) | (0.21, 0.31, 0.68) | O2 (2i) | (0.79, 0.31, 0.32) |
| O3 (2i) | (0.71, 0.81, 0.68) | O4 (2i) | (0.29, 0.81, 0.32) |
| O5 (2i) | (0.24, 0, 0.82) | O6 (2i) | (0.74, 0, 0.82) |

sible up to 3 GPa, refinement of Li and O coordinates becomes extremely challenging in the heavily distorted triclinic phase. To simplify this problem, a series of positional constraints were imposed in the high pressure phase. Li positions were refined for the *C2/m* structure (0 < P < 3 GPa), but were left fixed at their P = 2.8 GPa values for the *P-1* structure (3 < P < 10 GPa). O positions were refined for the *P-1* structure, but their relative changes in position were constrained by symmetry (i.e. we adopt O positional constraints similar to the low pressure monoclinic phase). Varying, or even completely releasing these constraints, did not change the goodness of fit, although it did result in significant convergence problems. In the future, we propose that the use of anomalous x-ray diffraction, or a local structural probe such as x-ray absorption fine structure (XAFS), may be helpful for fully resolving these issues.

## ANALYSIS OF THE RIXS SPECTRA

The high pressure RIXS spectra were analyzed using a similar approach to that employed by Gretarsson et al in previous analysis of $Na_2IrO_3$ and $\alpha$-$Li_2IrO_3$ at ambient pressure [16]. In particular, each spectrum was broken down into three main contributions: (i) the elastic line ($\Delta$E = 0), which was modeled by a resolution-limited pseudo-Voigt function (FWHM = 110 meV), (ii) the background continuum arising from particle-hole excitations, which was modeled by a step function, and (iii) the *d-d* excitations arising from intra-$t_{2g}$ transitions, which were modeled by a series of two (P < 2 GPa) to three (P > 2 GPa) Gaussian peaks.

At low pressure, a two *d-d* peak model is sufficient to fit the data very well. Since the previously reported non-cubic crystal field splitting in $\alpha$-$Li_2IrO_3$ ($\sim$ 110 meV) [16] is too small to be resolved in the current experimental setup, one would expect to observe a single *d-d* peak at ambient pressure. The observation of two peaks, split by $\sim$0.5 eV, implies a significant increase in non-cubic crystal field splitting. This could still be interpretted within a localized electron framework, but clearly indicates a breakdown of the $J_{eff}$ = 1/2 picture. At minimum, this spectrum implies the need to adopt a localized pseudospin 1/2 model more appropriate to the large $\Delta$ limit [17].

At higher pressures, the quality of the two *d-d* peak fit becomes significantly worse. This effect first becomes noticeable at P $\sim$ 2 GPa, but becomes much more problematic above 3 GPa. This issue can be solved by intro-

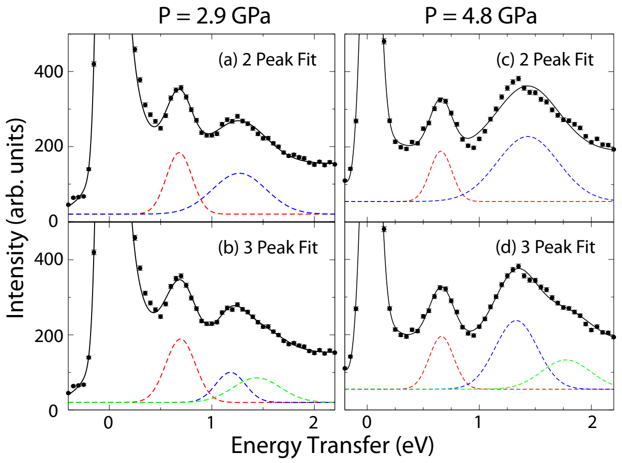


FIG. 4: (Color online) Analysis of RIXS spectra collected at (a,b) P = 2.9 GPa and (c,d) P = 4.8 GPa. These spectra have been fit to two different models, allowing for either: (a,c) two possible intra-$t_{2g}$ transitions [as would be appropriate for a localized $J_{eff}$ = 1/2 or S = 1/2 model], or (b,d) three possible intra-$t_{2g}$ transitions [as would be appropriate for a QMO-based model]. At higher pressures, the three peak model begins to provide a much more accurate description of the experimental data. The solid black lines represent the best fit obtained from a given model, while the dashed red, blue, and green lines represent the individual fit components associated with the intra-$t_{2g}$ transitions.

ducing a third *d-d* peak, which accounts for the increasingly asymmetric lineshape of the higher energy inelastic feature. A comparison of the two and three peak models is provided in Supplemental Figure 4. The relative positions of the three *d-d* peaks can be constrained using a QMO-based model, which reduces the number of adjustable parameters without significantly decreasing the quality of the fit. In terms of the nearest-neighbor ($t'_1$) and next-nearest-neighbor ($t'_2$) oxygen-mediated hopping parameters, the positions of the three peaks in the QMO model can be defined as $E_1 = t'_1 + 3t'_2$, $E_2 = 3t'_1 + 3t'_2$, and $E_3 = 4t'_1 + 4t'_2$.

We note one additional feature of the high pressure RIXS spectrum, which is an anomalous broadening of the elastic line that occurs in the vicinity of the structural transition at P $\sim$ 3 GPa. As shown by the representative spectra provided in Figure 3 of the main text, there is a clear increase in the low-lying inelastic spectral weight ($\Delta E < 0.3$ eV) which peaks at P = 2.9 GPa. This effect extends $\sim$1 GPa on either side of the transition, and can be observed on both increasing and decreasing pressure. The origin of this low-lying inelastic scattering remains an open question, and is a subject which requires further experimental investigation with higher energy resolution in the future.


[1] J. S. Smith and S. Desgreniers, J. Synch. Rad. **16**, 83 (2009).

[2] A. C. Larson and R. B. Van Dreele, Los Alamos National Laboratory Report LAUR 86-748 (2000).

[3] K. Koepernik and H. Eschrig, Phys. Rev. B **59**, 1743 (1999).

[4] D. Figgen, K. A. Peterson, M. Dolg, and H. Stoll, J. Chem. Phys. **130**, 164108 (2009).

[5] T. H. Dunning, J. Chem. Phys. **90**, 1007 (1989).

[6] K. Pierloot, B. Dumez, P.-O. Widmark, and B. O. Roos, Theoretica chimica acta **90**, 87 (1995).

[7] P. Fuentealba, H. Preuss, H. Stoll, and L. V. Szentply, Chemical Physics Letters **89**, 418 (1982).

[8] H. J. Werner, P. J. Knowles, G. Knizia, F. R. Manby, and M. Schütz, Wiley Rev: Comp. Mol. Sci. **2**, 242 (2012).

[9] H.-J. Werner and P. J. Knowles, J. Chem. Phys. **89**, 9 (1988).

[10] P. J. Knowles and H.-J. Werner, Theor. Chim. Acta **84**, 95 (1992).

[11] A. Berning, M. Schweizer, H.-J. Werner, P. J. Knowles, and P. Palmieri, Mol. Phys. **98**, 1823 (2000).

[12] V. M. Katukuri, K. Roszeitis, V. Yushankhai, A. Mitrushchenkov, H. Stoll, M. van Veenendaal, P. Fulde, J. van den Brink, and L. Hozoi, Inorganic Chemistry **53**, 4833 (2014).

[13] N. F. Mott, *Metal-Insulator Transitions* (Taylor & Francis Ltd., London, 1990).

[14] N. F. Mott, in *Festkörperproblems XIX*, edited by J. Treusch (Vieweg, Braunschweig, 1979), p. 331.

[15] M. J. O'Malley, H. Verweij, and P. M. Woodward, J. Solid State Chem. **181**, 1803 (2008).

[16] H. Gretarsson, J. P. Clancy, X. Liu, J. P. Hill, E. Bozin, Y. Singh, S. Manni, P. Gegenwart, J. Kim, A. H. Said, et al., Phys. Rev. Lett. **110**, 076402 (2013).

[17] S. Bhattacharjee, S.-S. Lee, and Y. B. Kim, New J. Phys. **14**, 073015 (2012).
